# Supplementary material for: Schmidt modes in the angular spectrum of bright squeezed vacuum
Source: arXiv:1410.6658 source file (2014-10-24)
Supplement: Supplementary file 1 [file supplementary_Bloch6.pdf]

# Supplementary information: Schmidt modes in the angular spectrum of bright squeezed vacuum

P. Sharapova,[1] A. M. Pérez,[2] O. V. Tikhonova,[1,3] and M. V. Chekhova[2,1]

[1] *Physics Department, Moscow State University, Leninskiye Gory 1-2, Moscow 119991, Russia*
[2] *Max-Planck Institute for the Science of Light, Guenther-Scharowsky-Str. 1 / Bau 24, Erlangen D-91058, Germany*
[3] *Skobeltsyn Institute of Nuclear Physics, Lomonosov Moscow State University, Moscow 119234, Russia*

Here we provide additional information on the material presented in the main paper. Section A considers the details of Schmidt modes calculation for the two-crystal scheme. Section B contains the derivation of the photon-number covariance in terms of plane waves. Section C describes the situation where double-Gaussian approximation can be used, and Section D is devoted to the case of strong anisotropy, where one-dimensional description is sufficient.

PACS numbers: 42.65.Lm, 42.65.Yj, 42.50.Lc

## A. The two-crystal scheme.

In all experiments described in the main text, PDC is obtained by placing two crystals one after another, usually with the optic axes tilted symmetrically with respect to the pump direction. Such a configuration, used already in the early papers on squeezing [1], allows one to reach high parametric gain without strong walk-off effect. However, the description of the two-dimensional spatial spectrum of its PDC emission has been never done before.

The two-crystal case is more complicated to describe than the single-crystal one. The latter, under certain conditions, allows the two-photon amplitude (TPA) to be written in the double-Gauss approximation and further factored in two one-dimensional distributions. In the two-crystal case, due to the interference between the radiation from different crystals, the TPA contains multiple maxima and minima and therefore cannot be described within the framework of the double-Gauss model. Moreover, the geometry obviously has cylindrical symmetry and does not allow factorization of the TPA in the horizontal and vertical parts. This immediately dictates using the Laguerre-Gauss basis for the TPA Schmidt decomposition.

The two-crystal scheme we consider is shown in Fig. 1. Two crystals of length $L$ are separated by an air gap of length $d$ and pumped by a Gaussian pump with the beam waist described by the parameter $\sigma$. The full width at half maximum (FWHM) of the pump intensity distribution, $2\sqrt{\ln 2}\sigma$, is assumed to be much larger than the transverse walk-off distance in a single crystal. This allows one to neglect the transverse walk-off and makes the system cylindrically symmetric. We also assume frequency degeneracy, i.e., that the signal and idler frequencies are equal to $\omega_s = \omega_p/2$, with $\omega_p$ denoting the frequency of the pump.

The TPA $F(\mathbf{q}_s, \mathbf{q}_i)$ for this scheme can be written in the form [2–4]

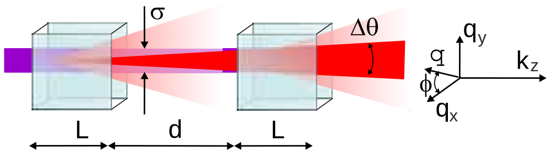


FIG. 1. The two-crystal scheme and the basic notation. The angular width of radiation from the first crystal amplified in the second crystal, $\Delta\theta$, is determined by the ratio $\sigma/(2L+d)$, where $\sigma$ characterizes the pump width, $L$ is the crystal length and $d$ the distance between the crystals. The transverse components of the wavevectors are denoted by $\mathbf{q}$.

$$\begin{aligned} F(\mathbf{q}_s, \mathbf{q}_i) &= C \exp\{-\frac{\sigma^2(\mathbf{q}_s+\mathbf{q}_i)^2}{2}\} \\ &\times \mathrm{sinc}(\frac{L(\mathbf{q}_s-\mathbf{q}_i)^2}{4k_p}) \exp(\frac{-iL(\mathbf{q}_s-\mathbf{q}_i)^2}{4k_p}) \\ &\times \cos(\frac{L(\mathbf{q}_s-\mathbf{q}_i)^2}{4k_p} + \frac{\delta n k_s}{n_s} + \frac{d(\mathbf{q}_s^{air}-\mathbf{q}_i^{air})^2}{4k_p^{air}}) \\ &\times \exp\{i(\frac{L(\mathbf{q}_s-\mathbf{q}_i)^2}{4k_p} + \frac{\delta n k_s}{n_s} + \frac{d(\mathbf{q}_s^{air}-\mathbf{q}_i^{air})^2}{4k_p^{air}})\}, \end{aligned} \quad (1)$$

where $C$ is the normalization constant, $k_{p,s}^{air} = n_{p,s}^{air}\frac{\omega_{p,s}}{c}$, $n_{p,s,i}^{air}$ are the refractive indices for the pump, signal and idler radiation in the air gap between the crystals, $\delta n = n_p^{air} - \frac{1}{2}(n_s^{air} + n_i^{air})$ and $\mathbf{q}_{s,i}^{air}(\mathbf{q}_{s,i})$ are the transverse components of the wave vectors of the signal and idler beams in the air gap (crystal). In the cylindrical frame of reference, they are characterized by their absolute values $q_{s,i}$ and azimuthal angles $\phi_{s,i}$: $\mathbf{q}_{s,i} = (q_{s,i}, \phi_{s,i})$. For small angles of emission, $\frac{(\mathbf{q}_s^{air}-\mathbf{q}_i^{air})^2}{4k_p^{air}} \approx n_s\frac{(\mathbf{q}_s-\mathbf{q}_i)^2}{4k_p}$. In this case the TPA (1) depends on four polar coordinates describing the transverse wave vectors of the signal and idler beams. The key point of the cylindrical symmetry is that the TPA depends not separately on the angles $\phi_s$ and $\phi_i$ but only on their difference $(\phi_s - \phi_i)$. This immediately enables an explicit Schmidt decomposition

of the TPA as it was described in Eqs. (3,4) of the main text.

At the same time, in the Cartesian frame of reference the explicit Schmidt decomposition can hardly be performed in full dimensionality. For this reason different approximations should be used to simplify this procedure. One of them is appropriate if the distance between the crystals is small compared to the period of the interference pattern observed when one of the crystals is moved (36mm [2]), then the approximation of a single crystal of double length can be used. In this case, the double-Gauss approximation can be applied and the Schmidt decomposition of the TPA can be provided separately in each (x or y) direction. This method is described below in Section C. Another simplification is appropriate if the anisotropy plays an important role. In such a case only a single dimension needs to be considered, the one in which the spatial walk-off takes place. Whenever all important effects are associated with anisotropy they can be taken into account under such 1D approximation. Thus the problem of the Schmidt decomposition can be solved by different means, and as soon as it is solved, our analytical approach leads straightforward to the final results. Thus our method based on collective Schmidt modes can be successfully used for different experimental schemes.

### B. Plane-wave solutions.

In the general case, the Schmidt decomposition of the TPA (1) can be performed in the cylindrical frame of reference taking into account that $\mathbf{q}_s\mathbf{q}_i = q_s q_i \cos(\phi_s - \phi_i)$ and using the fact that the TPA depends only on the difference $\phi_s - \phi_i$ and this dependence is periodic. Such a feature is a direct consequence of the azimuthal symmetry of PDC radiation in the scheme we use and leads to the invariance of the radiation intensity to the azimuthal angle. Under these conditions it is possible to introduce new collective photon creation operators $A^\dagger_{mn}$ , $B^\dagger_{mn}$ as described in the main text [Eq. (7)]. These operators are responsible for the creation of a photon in a certain Schmidt mode characterized by its own spatial distribution. Since usually the description not only in terms of the Schmidt modes but also in the framework of plane-wave operators is needed, further we find the solution for these operators and calculate some measurable quantities. Using the expression for the Hamiltonian in terms of $A^\dagger_{mn}$ and $B^\dagger_{mn}$ given by Eq (6) of the main text, the Heisenberg equation for plane-wave operators $a_{s,i}$ can be written in the form

$$\frac{da_{\mathbf{q}_{s,i}}}{dt} = \Gamma \sum_{mn} \sqrt{\lambda_{mn}} \frac{u_{mn}(q_{s,i})}{\sqrt{q_{s,i}}} [A^\dagger_{mn} e^{-in\phi_{s,i}} + B^\dagger_{mn} e^{in\phi_{s,i}}] \quad (2)$$

Here we use the fact that $u_{mn}(\xi) = v_{mn}(\xi)$ due to the invariance of TPA (1) to the $\mathbf{q_s} \leftrightarrow \mathbf{q_i}$ exchange.

With an account for the time-dependent expression of the Schmidt mode operators $A^\dagger_{mn}$, $B^\dagger_{mn}$ found in the main text, after introducing $S_{mn}(\phi) \equiv \frac{1}{2}[B^{in}_{mn} e^{-in\phi} + A^{in}_{mn} e^{in\phi}]$ we obtain the solution of (2) in the form

$$a^{out}_{\mathbf{q}_{s,i}} = a^{in}_{\mathbf{q}_{s,i}} + \sum_{mn} \frac{u_{mn}(q_{s,i})}{\sqrt{q_{s,i}}} \times [S^\dagger_{mn}(\phi_{s,i}) \sinh(\sqrt{\lambda_{mn}}G) + S_{mn}(\phi_{s,i})(\cosh(\sqrt{\lambda_{mn}}G) - 1)]. \quad (3)$$

From this solution, we calculate the mean photon number, for example, for the signal beam by averaging $[a^{out}_{\mathbf{q}_s}]^\dagger a^{out}_{\mathbf{q}_s}$ over the vacuum state:

$$\langle N_s(\mathbf{q}_s)\rangle = \sum_{mn} \frac{|u_{mn}(q_s)|^2}{q_s} (\sinh[G\sqrt{\lambda_{mn}}])^2. \quad (4)$$

We also calculate the covariance of the photon numbers,

$$\mathrm{Cov}(\mathrm{N_s}(\mathbf{q_s}), \mathrm{N_i}(\mathbf{q_i})) = = \langle N_s(\mathbf{q}_s) N_i(\mathbf{q}_i)\rangle - \langle N_s(\mathbf{q}_s)\rangle\langle N_i(\mathbf{q}_i)\rangle. \quad (5)$$

It should be emphasized that while the Schmidt modes depend on the azimuthal angles of signal and idler photons, the mean photon numbers demonstrate independence on them. At the same time, the covariance depends on the combination $(\phi_s - \phi_i)$, which evidently shows correlation between the signal and idler photons with transverse wave vectors of the same or opposite directions ($\cos(\phi_s - \phi_i) = 0, \pi$, corresponding to auto- and cross-correlations, respectively):

$$\begin{aligned}
&\mathrm{Cov}(\mathrm{N_s}(\mathbf{q_s}), \mathrm{N_i}(\mathbf{q_i})) = \\
&|\sum_{mn} \frac{v_{mn}(q_i) u_{mn}(q_s)}{\sqrt{q_i q_s}} \sinh[\sqrt{\lambda_{mn}}G] \times \\
&(\cosh[\sqrt{\lambda_{mn}}G] - 1) \cos[n(\phi_s - \phi_i)]|^2 \\
&+2\mathrm{Re}[\sum_{mn} \frac{v^*_{mn}(q_i) u^*_{mn}(q_s)}{\sqrt{q_i q_s}} \sinh[\sqrt{\lambda_{mn}}G] \times \\
&\times(\cosh[\sqrt{\lambda_{mn}}G] - 1) \cos[n(\phi_s - \phi_i)] \times \\
&\sum_{mn} \frac{v_{mn}(q_i) u_{mn}(q_s)}{\sqrt{q_i q_s}} \sinh[\sqrt{\lambda_{mn}}G] \cos[n(\phi_s - \phi_i)]] \\
&+|\sum_{mn} \frac{v_{mn}(q_i) u_{mn}(q_s)}{\sqrt{q_i q_s}} \sinh[\sqrt{\lambda_{mn}}G] \cos[n(\phi_s - \phi_i)]|^2 \\
&+\sum_{mn} \frac{|v_{mn}(q_i)|^2 |u_{mn}(q_s)|^2}{q_i q_s} (\sinh[\sqrt{\lambda_{mn}}G])^4 \times \\
&\times(1 + 2\cos[2n(\phi_s - \phi_i)]) + \\
&|\sum_{mn} \frac{v^*_{mn}(q_i) u_{mn}(q_s)}{\sqrt{q_i q_s}} (\sinh[\sqrt{\lambda_{mn}}G])^2 \cos[n(\phi_s - \phi_i)]|^2 \quad (6)
\end{aligned}$$

However, if only emission within a certain plane is analyzed (which can be achieved in experiment by using a

horizontal or a vertical slit in front of the CCD or using only a single vertical or horizontal row of the CCD pixels), the covariance takes a simpler form and depends on only two variables $q_s$ and $q_i$.

### C. Cartesian frame and double-Gauss approximation

The general expression of TPA (1) cannot be written as a product of one-dimensional TPAs in the Cartesian frame of reference, for instance one depending on the $x$ and the other one depending on the $y$ wave vector components. Because of this, the problem can be solved analytically only under some approximations.

For instance, if the distance between the two crystals is small and the crystals have optic axes tilted oppositely, one can consider such a system as one crystal of double length. Then the double-Gauss approximation, in which the *sinc*-term of the TPA is approximated by a Gaussian function with suited parameters, can be used. The amplitude can then be factored in two terms, each one depending only on the $x$ or $y$ components of $\mathbf{q}_s$ and $\mathbf{q}_i$,

$$F(\mathbf{q}_s, \mathbf{q}_i) = F_1(q_{sx}, q_{ix}) F_2(q_{sy}, q_{iy}). \quad (7)$$

In this case, the Schmidt decomposition for $x$ and $y$ directions can be provided independently on each other,

$$F(\mathbf{q}_s, \mathbf{q}_i) = \sum_n \sqrt{\lambda_n} u_n(q_{sx}) v_n(q_{ix}) \times \sum_m \sqrt{\tilde{\lambda}_m} \tilde{u}_m(q_{sy}) \tilde{v}_m(q_{iy}). \quad (8)$$

As a result, the TPA can be represented as the decomposition in two-dimensional Schmidt modes, $U_{nm}(\mathbf{q}_s) = u_n(q_{sx})\tilde{u}_m(q_{sy})$, $V_{nm}(\mathbf{q}_i) = v_n(q_{ix})\tilde{v}_m(q_{iy})$, depending on the signal or idler variables only:

$$F(\mathbf{q}_s, \mathbf{q}_i) = \sum_{nm} \sqrt{\lambda_n \tilde{\lambda}_m} U_{nm}(\mathbf{q}_s) V_{nm}(\mathbf{q}_i). \quad (9)$$

It should be noticed that since the anisotropy is not taken into account and the pump is axially symmetric, the eigenmodes and eigenvalues for $x$ and $y$ directions are identical:

$$u_n(\xi) = \tilde{u}_n(\xi), v_n(\xi) = \tilde{v}_n(\xi), \lambda_n = \tilde{\lambda}_n. \quad (10)$$

Then we can introduce new collective photon creation operators $A^\dagger_{mn}$, $B^\dagger_{mn}$,

$$A^\dagger_{mn} = \int d\mathbf{q}_s U_{mn}(\mathbf{q}_s) a^\dagger_{\mathbf{q}_s},$$
$$B^\dagger_{mn} = \int d\mathbf{q}_i V_{mn}(\mathbf{q}_i) a^\dagger_{\mathbf{q}_i}, \quad (11)$$

which provide the diagonalization of the initial Hamiltonian and allow one to obtain the time-depending solution not only for Schmidt modes but also for the plane-wave operators. From the expressions obtained for the plane-wave operators, we can calculate the mean photon number, as well as the variance of the photon-number difference in the signal and idler beams, $\mathrm{Var}(N_s - N_i) \equiv \langle (N_s - N_i)^2 \rangle - \langle N_s - N_i \rangle^2$, the correlation function $G^{(2)}_{is} \equiv \langle N_s N_i \rangle$, and its normalized value, $g^{(2)}_{is} \equiv \frac{G^{(2)}_{is}}{\langle N_s \rangle \langle N_i \rangle}$. In full dimensionality the mean number of photons for the signal beam (and analogical for the idler beam) takes the form

$$N_s(q_{sx}, q_{sy}) = \sum_{nm} |u_n(q_{sx})|^2 |u_m(q_{sy})|^2 (\sinh[\sqrt{\lambda_n \lambda_m} G])^2. \quad (12)$$

But if only one-dimensional distribution is analyzed in experiment by fixing $q_{iy} = q_{sy} = 0$ (using a slit), it is given by

$$N_s(q_{sx}) = \sum_{nm} |u_n(q_{sx})|^2 |u_m(0)|^2 (\sinh[\sqrt{\lambda_n \lambda_m} G])^2. \quad (13)$$

Moreover, in the case when the number of modes is sufficiently small and consequently their weights drop sharply with the increase of $n$ (which was realized in experiment), one can restrict the sum over $m$ to only the first term and the signal takes a simpler form,

$$N_s(q_{sx}) = \sum_n |u_n(q_{sx})|^2 |u_0(0)|^2 (\sinh[\sqrt{\lambda_n \lambda_0} G])^2. \quad (14)$$

Under such conditions the variance of the photon number difference can be represented as

$$\mathrm{Var}(N_s - N_i) = \mathrm{Var}(N_s) + \mathrm{Var}(N_i) - 2\mathrm{Cov}(N_s, N_i), \quad (15)$$

where

$$\mathrm{Var}(N_s) = |u_0(0)|^4 (|\sum u_n u_n \sinh[\Lambda_n](\cosh[\Lambda_n] - 1)|^2 + 2\mathrm{Re}[\sum u^*_n u^*_n \sinh[\Lambda_n](\cosh[\Lambda_n] - 1) \sum u_n u_n \sinh[\Lambda_n] + |\sum u_n u_n \sinh[\Lambda_n]|^2 + |\sum u^*_n u_n (\sinh[\Lambda_n])^2|^2 + 3 \sum |u_n|^2 |u_n|^2 (\sinh[\Lambda_n])^4) + |u_0(0)|^2 \langle N_s \rangle, \quad (16)$$

$$\mathrm{Var}(N_i) = |v_0(0)|^4 (|\sum v_n v_n \sinh[\Lambda_n](\cosh[\Lambda_n] - 1)|^2 + 2\mathrm{Re}[\sum v^*_n v^*_n \sinh[\Lambda_n](\cosh[\Lambda_n] - 1) \sum v_n v_n \sinh[\Lambda_n] + |\sum v_n v_n \sinh[\Lambda_n]|^2 + |\sum v^*_n v_n (\sinh[\Lambda_n])^2|^2 + 3 \sum |v_n|^2 |v_n|^2 (\sinh[\Lambda_n])^4) + |v_0(0)|^2 \langle N_i \rangle, \quad (17)$$

$$\mathrm{Cov}(N_s,N_i) = |u_0(0)|^2|v_0(0)|^2(|\sum v_n u_n \sinh[\Lambda_n](\cosh[\Lambda_n]-1)|^2 +2\mathrm{Re}[\sum v_n^* u_n^* \sinh[\Lambda_n](\cosh[\Lambda_n]-1)\sum v_n u_n \sinh[\Lambda_n] +|\sum v_n u_n \sinh[\Lambda_n]|^2 + |\sum v_n^* u_n (\sinh[\Lambda_n])^2|^2 +3\sum |v_n|^2|u_n|^2(\sinh[\Lambda_n])^4), \quad (18)$$

with $u_n = u_n(q_{sx}), v_n = v_n(q_{ix})$ and $\Lambda_n = G\sqrt{\lambda_n\lambda_0}$. It should be noticed that this approximation works rather well for two closely placed crystals. Indeed, the theoretical results obtained by such a way fit very well the experimental curves (see Fig. 1 of the main text).

### D. Anisotropy effect

If the pump diameter is small, or the crystal is long, it is necessary to take into account the spatial walk-off. This breaks down the axial symmetry of the problem. However, in some cases, it is enough to take into account not the full two-dimensional angular spectra but only a single dimension. For instance, when the walk-off effect is described, it is sufficient to consider only the plane of the optic axis. The corresponding TPA is described by the expression obtained in [5] but including non-zero distance between the crystals. For the 'compensating' geometry, in which the two crystals have optic axes tilted oppositely, the TPA can be written as

$$F(\theta_s,\theta_i) = \exp[-\frac{\sigma^2(\Delta_\perp\cos\rho+\Delta_\parallel\sin\rho)^2}{2}]\exp[-i\frac{L}{2}\xi]\mathrm{sinc}[\frac{L}{2}\xi] +\exp[-\frac{\sigma^2(\Delta_\perp\cos\rho-\Delta_\parallel\sin\rho)^2}{2}]\exp[i\frac{L}{2}\eta]\mathrm{sinc}[\frac{L}{2}\eta] \times\exp[i(L\Delta_\parallel + d\Delta_\parallel^{air})], \quad (19)$$

where $\rho$ is the walk-off angle, $\Delta_\parallel = k_p - k_s\cos\theta_s - k_i\cos\theta_i$ and $\Delta_\parallel^{air} = k_p^{air} - k_s^{air}\cos(n_s\theta_s) - k_i^{air}\cos(n_i\theta_i)$ are longitudinal mismatches in the crystal and in the air gap, respectively, $\Delta_\perp = k_s\sin\theta_s + k_i\sin\theta_i$ is the transverse mismatch, $\xi = \Delta_\parallel - \Delta_\perp\tan\rho$, $\eta = \Delta_\parallel + \Delta_\perp\tan\rho$.

For 'non-compensating' geometry, in which the optic axes are parallel in both crystals, we have

$$F(\theta_s,\theta_i) = \exp[-\frac{\sigma^2(\Delta_\perp\cos\rho+\Delta_\parallel\sin\rho)^2}{2}]\exp[-i\frac{L}{2}\xi]\mathrm{sinc}[\frac{L}{2}\xi] +\exp[-\frac{\sigma^2(\Delta_\perp\cos\rho+\Delta_\parallel\sin\rho)^2}{2}]\exp[-i\frac{L}{2}\xi]\mathrm{sinc}[\frac{L}{2}\xi] \times\exp[i(L\Delta_\parallel + d\Delta_\parallel^{air})]. \quad (20)$$

In this case, the one-dimensional approximation reflects the main features of the system and allows one to describe the behaviour of the signal not only qualitatively but also quantitatively. Nevertheless, the consideration in full dimensionality without any approximations remains an important but difficult problem and will be a subject of our further investigation.


[1] P. Grangier, R. E. Slusher, B. Yurke, and A. LaPorta, PRL **59**, 2153 (1987).
[2] A. M. Pérez, T. Sh. Iskhakov, P. Sharapova, S. Lemieux, O. V. Tikhonova, M. V. Chekhova, and G. Leuchs, Optics Letters **39**, 2403 (2014).
[3] F. M. Miatto, T. Brougham, and A. M. Yao, Eur. Phys. J. D **66**, 183 (2012).
[4] D. N. Klyshko, JETP **104**, 2676 (1993).
[5] A. Pérez, A. Cavanna, F. Just, M. V. Chekhova, and G. Leuchs, Laser Physics Letters **10**, 125201 (2013).
